# Supplementary material for: Quantitative Diffractometric Biosensing
Source: arXiv:2011.15052 source file (2020-11-30)
Supplement: Supplementary file 1 [file Blickenstorfer_et_al_SM.pdf]

# Quantitative diffractometric biosensing

Yves Blickenstorfer,[1,*] Markus Müller,[2] Roland Dreyfus,[1] Andreas Michael Reichmuth,[1] Christof Fattinger,[3,†] and Andreas Frutiger[1,‡]

[1] *Laboratory of Biosensors and Bioelectronics, Institute of Biomedical Engineering, ETH Zürich, 8092 Zürich, Switzerland*
[2] *Condensed Matter Theory Group, Paul Scherrer Institute, 5232 Villigen, Switzerland*
[3] *Roche Pharma Research and Early Development, Roche Innovation Center Basel, 4070 Basel, Switzerland*

## I. TWO DIMENSIONAL COUPLED MODE THEORY FOR WEAK COUPLING

One-dimensional ideal coupled mode theory has been described in detail in [1]. Here we extend it to two dimensions, by allowing the propagation vector $\vec{\beta}$ to be unrestricted in the 2d dielectric plane (whereas Ref. [1] restricted $\vec{\beta}$ to be normal to the grating), and by discussing beams of finite extent transverse to the beam. We choose coordinates such that the $z$-axis is perpendicular to the dielectric plane, while the $x$-axis is normal to the grating. Note that in the case of a freely propagating mode $\vec{\beta}$ is the projection of the 3d propagation vector $\vec{k}$ onto the dielectric plane (Figure 3). Apart from these modifications the formalism remains the same: For the total electric field one writes the ansatz

$$\vec{E}_{\text{tot}} = c_{\text{in}}\vec{E}_{\text{b,in}} + c_{\text{out}}\vec{E}_{\text{b,out}}, \tag{18}$$

where $\vec{E}_{\text{b,in/out}}$ are the fields of an in- or outgoing beam of normalized power and finite lateral beamshape. The amplitudes $c_{\text{in/out}}(x,y)$ vary slowly in the dielectric plane, as described by coupled mode equations (cf. Marcuse (Eqns. (3.2-34) and (3.2-35)). For a guided beam, we write its normalized electric field as

$$\vec{E}_{\text{b},\vec{\beta},s/p}(x,y,z) = \mathcal{N}\vec{E}_{\vec{\beta},s/p}(z)\,A(\vec{r}_\perp)\exp\left(i\vec{\beta}\cdot\vec{r}\right), \tag{19}$$

where $\vec{E}_{\vec{\beta},s/p}(z)$ is the electric field (not normalized) of the dominant mode of polarization s or p in the beam. We recall that a mode with electric field $\vec{E}_{\vec{\beta},s/p}(z)\exp\left(i\vec{\beta}\cdot\vec{r}\right)$ is an exact solution of Maxwell's solution for the ideal structure. $A(\vec{r}_\perp)$ describes the envelope perpendicular to the propagation direction ($\vec{r}_\perp = \vec{r}_{xy} - \frac{\vec{\beta}}{|\vec{\beta}|}\left(\vec{r}_{xy}\cdot\frac{\vec{\beta}}{|\vec{\beta}|}\right)$), where $\vec{r}_{xy} \equiv x\vec{e}_x + y\vec{e}_y$ is the position vector in the plane. For simplicity, we assume a rectangular beam of width $w_b$,

$$A(\vec{r_\perp}) = \Theta(w_b/2 - |\vec{r_\perp}|), \tag{20}$$

where $\Theta$ is the Heaviside Theta function. Finally, the normalization constant $\mathcal{N}$ is chosen such as to normalize the total power of the beam to the arbitrarily chosen value $P$, as discussed in Supplementary Information Section III below.

In the case of an outgoing guided beam, $w_b$ is chosen as the width of the molecular assembly projected onto the line perpendicular to $\beta$ (in the dielectric plane) (Figure 6d).

In the case of a freely propagating beam the field distribution is very similar

$$\vec{E}_{\text{b},\vec{\beta},s/p}(x,y,z) = \mathcal{N}\vec{E}_{\vec{\beta},s/p}(z)\,A(\vec{r}_\perp)\exp\left(i\vec{\beta}\cdot\vec{r}\right), \tag{21}$$

but now with $\vec{r}_\perp = \vec{r} - \frac{\vec{k}}{|\vec{k}|}\left(\vec{r}\cdot\frac{\vec{k}}{|\vec{k}|}\right)$, where $\vec{k} = \vec{\beta} + k_z\vec{e}_z$ is the 3d propagation vector.[2] For an incident beam we take a circular shape of radius $w_b/2$ as described by Eq. (20). For a freely propagating outgoing beam we take $A(\vec{r}_\perp)$ to be the indicator function of the grating area projected onto a plane perpendicular to $\vec{k}$ (that is, $A = 1$ in the projected area, and $A = 0$ outside.) For non-normal outgoing beams the indicator function will assume the shape of an ellipse for a grating of circular shape.

To determine the power transfer between two modes - *i.e.* their mutual coupling - one needs to compute the amplitude $c_{\text{out}}$ of the outgoing mode as a function of the amplitude of the incident mode $c_{\text{in}}$. A priori, this requires solving integrodifferential equations (cf. Eqns. 3.2-49 and 3.2-50 in Ref. [1]). However, in our case the coupling due to the biosensor is weak, and thus, the amplitude $c_{\text{in}}$ can be taken to be constant over the grating (negligible power loss), being the dominant contribution to the total field ($\vec{E}_{\text{tot}} \approx \vec{E}_{\text{b,in}}$). Furthermore, we are only interested in the power coupled into the specific outgoing mode with propagation direction defined by the grating equation,

$$\vec{\beta}_{\text{out}} = \vec{\beta}_{\text{in}} \pm \left|\vec{\beta}_g\right|\vec{e}_x, \tag{22}$$

where $\left|\vec{\beta}_g\right| = 2\pi/\Lambda$ is the grating wavevector and $\Lambda$ is the grating period. With these simplifying assumptions, the mode coupling equations reduce to one differential equation for the out-going amplitude of interest $c_{\text{out}}$.[3]

$$\frac{dc_{\text{out}}}{dx} = -\tilde{K}_{\text{out,in}}(x)c_{\text{in}}, \tag{23}$$

* A. Frutiger and Y. Blickenstorfer contributed equally to this work.
† christof.fattinger@gmail.com
‡ afrutig@ethz.ch

where

$$\tilde{K}_{\mathrm{out,in}}(x) = \frac{\omega\varepsilon_0}{4iP}\int_0^{\infty} dz \int_{-\infty}^{\infty} \left(n_m(x,y,z)^2 - n_c^2\right)$$
$$\left(\vec{E}^*_{\mathrm{out,t}}\cdot\vec{E}_{\mathrm{in,t}} + \frac{n_c^2}{n_m(x,y,z)^2}\vec{E}^*_{\mathrm{out,n}}\cdot\vec{E}_{\mathrm{in,n}}\right) e^{i(\vec{\beta}_{\mathrm{in}}-\vec{\beta}_{\mathrm{out}})\vec{r}}dy \tag{24}$$

is the $x$-dependent coupling coefficient between the incident and the outgoing mode. $\varepsilon_0$ is the permittivity of vacuum. $n_m(x,y,z)$ is the refractive index distribution in the real (i.e. perturbed) system. In the above expression, $\vec{E}_{\mathrm{in,out}} \equiv \mathcal{N}\vec{E}_{\vec{\beta}}(z)A(\vec{r}_\perp)$ are the normalized, $z$-dependent electric fields appearing in Eqs. ((19) and (21)). The subscripts $t$ and $n$ stand for the tangential and normal components of the electric field with respect to the dielectric surface, respectively. The larger the field overlap in Eq. (24) the stronger the coupling. The coupling is strongest for modes with parallel field vectors, but vanishes for modes with mutually orthogonal directions of the $\vec{E}$ field, so that energy cannot be transferred between them. Our expressions differ from those in Ref. [1], because the coupled mode theory based on the ideal mode expansion discussed there is strictly valid for TE-modes only [4, 5]. The expression given above has been suggested by Ref. [6] to account for the inaccuracies of ideal coupled mode theory in the case of TM polarization, which does not properly satisfy the boundary conditions and thereby assigns an incorrect weight to the normal field components [4]. Ref. [6] suggested to adjust the ideal mode expansion to correct for the modified normal field strength within the perturbation region, accounting for Maxwell's boundary conditions, and we follow that approach here. Nevertheless, the resulting errors are negligible even for the original ideal mode expansion, if the refractive index difference between the ideal and the perturbed structure is small, as is the case for molecular gratings; and even for larger refractive index differences (as in the case of surface roughness) the error of this approximation is likely to be smaller than other uncertainties in a given experimental set-up.

### A. General normalization of beam electric fields

As indicated above, we normalize the field amplitudes of the beam fields in Eqs. ((19) and (21)) to a total power of $P$. The incident and outgoing power are then simply related to the amplitudes $c_{\mathrm{out/in}}$ by $P_{\mathrm{out/in}} = \left|c_{\mathrm{out/in}}\right|^2 P$. [7] The power carried by a beam is evaluated by the integral over its Poynting vector

$$P_\nu = \int\int_S \frac{1}{2}\vec{e}_n\cdot\left(\vec{E}_\nu \times \vec{H}^*_\nu\right) dS, \tag{25}$$

where $\nu$ indicates the incident or outgoing beam, and $\vec{H}_\nu$ is the magnetic field associated with that mode. In general, $S$ is any infinite two-dimensional plane that is not parallel to the beam propagation direction, and $\vec{e}_n$ is a unit vector normal to $S$.

Qualitatively, the total power is of course proportional to the crosssectional area $\mathcal{A}$ of the beam, as well as to a typical value of the electric field $\mathcal{E}$ in the center of the beam,

$$P \sim \mathcal{A}\mathcal{E}^2. \tag{26}$$

Accordingly, the normalization factors in Eqs (16 and 18) scale as

$$\mathcal{N} \sim \sqrt{\frac{P}{\mathcal{A}}}. \tag{27}$$

### B. Derivation of the diffraction efficiency

In this section, we derive the diffraction efficiency from Eqn. (23). We start by assuming the refractive index of the perturbation as constant. It is located on the dielectric surface and extends with a height $\tilde{f}(x,y)$ into the cover. $\tilde{f}(x,y)$ is called the perturbation function. The tilde indicates that this function is confined to an area of interest and is zero everywhere outside that region. Since the absolute value of this height is assumed to be much smaller than the wavelength, we can assume the electric field to be constant over the entire perturbation. Thus, to compute the coupling coefficient one can replace the integration over $z$ by the integrand evaluated at the interface from the cover side ($z = 0^+$) and multiply by the height:

$$\tilde{K}_{\mathrm{out,in}}(x) = \frac{\omega\varepsilon_0}{4iP}$$
$$\left(\vec{E}^*_{\mathrm{out,t}}(0)\cdot\vec{E}_{\mathrm{in,t}}(0) + \frac{n_c^2}{n_m^2}\vec{E}^*_{\mathrm{out,n}}(0)\cdot\vec{E}_{\mathrm{in,n}}(0)\right)$$
$$\left(n_m^2 - n_c^2\right)\int_{-\infty}^{\infty} \tilde{f}(x,y)e^{i(\vec{\beta}_{\mathrm{in}}-\vec{\beta}_{\mathrm{out}})\vec{r}}dy. \tag{28}$$

Note that we took the factors of the electric fields outside the integral, considering them constant over the area where $f(x,y)$ is non-zero, since the beam envelope is as wide as the grating, or wider.

It is now simple to integrate Eqn. (23) with respect to $x$. This yields the amplitude of the out-going beam at the location where the beam leaves the grating area:

$$\frac{c_{\mathrm{out}}}{c_{\mathrm{in}}} = \hat{K}\int_{-\infty}^{\infty}\int_{-\infty}^{\infty} \tilde{f}(x,y)e^{i(\vec{\beta}_{\mathrm{in}}-\vec{\beta}_{\mathrm{out}})\vec{r}}dxdy. \tag{29}$$

The expression is easily recognized as the two-dimensional Fourier transformation of the perturbation function multiplied by $\hat{K}$. $\hat{K}$ is the *constant coupling co-*

*efficient* which is independent of the perturbation function [1]:

$$\hat{K} = \frac{\omega\varepsilon_0}{4iP}$$
$$\left(\vec{E}^*_{\mathrm{out,t}}(0)\cdot\vec{E}_{\mathrm{in,t}}(0) + \frac{n_c^2}{n_m^2}\vec{E}^*_{\mathrm{out,n}}(0)\cdot\vec{E}_{\mathrm{in,n}}(0)\right)\left(n_m^2 - n_c^2\right). \tag{30}$$

For biosensing applications it makes sense to separate the factor $n_m^2 - n_c^2$, because the effective refractive index of the modulation, $n_m$, depends on the amount of bound biological mass. Hence, in the main manuscript we defined $K := \frac{\hat{K}}{(n_m^2 - n_c^2)}$ as the coupling coefficient. Since the total power of the beams is proportional to the squared amplitude $c_{\mathrm{in/out}}$ (Eqn. (6)), the diffraction efficiency is simply the square of the above ratio

$$\frac{P_{\mathrm{out}}}{P_{\mathrm{in}}} = \left|\frac{c_{\mathrm{out}}}{c_{\mathrm{in}}}\right|^2 = \left\langle\left|\hat{K}\int\int_A f(x,y)e^{i\left(\vec{\beta}_{\mathrm{in}}-\vec{\beta}_{\mathrm{out}}\right)\vec{r}}dA\right|^2\right\rangle, \tag{31}$$

where we made use of the fact that the perturbation function is finite only in area $A$. We have included an average $\langle ... \rangle$ over realizations of randomness, in case the perturbation function describes random fluctuations.

As mentioned above $\tilde{f}(x,y)$ is nonzero only in a finite area. Sometimes, it is convenient to express the perturbation as a function extending to infinity $f(x,y)$, however. The integral in Eqn. (29) can then be expressed by two different approaches. Either we limit the integration to the area of interest, as above, or we multiply $f(x,y)$ with a shape function

$$s(x,y) = \begin{matrix} 1, & \text{inside area of interest} \\ 0, & \text{outside area of interest} \end{matrix} \tag{32}$$

to yield

$$\frac{P_{\mathrm{out}}}{P_{\mathrm{in}}} = \left\langle\left|\hat{K}\int_{-\infty}^{\infty}\int_{-\infty}^{\infty} s(x,y)f(x,y)e^{i\left(\vec{\beta}_{\mathrm{in}}-\vec{\beta}_{\mathrm{out}}\right)\vec{r}}dxdy\right|^2\right\rangle. \tag{33}$$

Eqns. (31) and (33) are the general expressions that need to be evaluated to compute the diffraction efficiency for a perturbation function and a certain coupling coefficient of the optical configuration. Eqn. (31) is more convenient to analyze the scattering from surface roughness whereas Eqn. (33) is appropriate when computing the diffraction at a regular grating.

## II. EXAMPLES OF TWO-DIMENSIONAL COUPLED MODE THEORY APPLIED TO TWO DIMENSIONAL PERTURBATIONS

In this section we evaluate Eqns. (31) and (33) for different perturbation functions. For the analysis of diffractometric sensors we should discuss both periodic and random perturbation functions. Periodic perturbations arise due to analytes binding to the structured sensor surface. Random perturbations instead describe surface roughness or nonspecific binding. These random processes are responsible for the speckle background on the detector.

### A. Periodic perturbation functions

In diffractometric biosensors, the signal is caused by a periodic perturbation of the refractive index due to bound analyte molecules. In order to evaluate the diffraction efficiency for any incident and outgoing modes it is convenient to use Eqn. (33). It can be rewritten as a convolution of the Fourier transforms of the shape and the perturbation function. We define the two-dimensional Fourier transform as

$$\hat{f}\left(k_x,k_y\right) := \int_{-\infty}^{\infty}\int_{-\infty}^{\infty} f(x,y)e^{-i(k_x x + k_y y)}dxdy, \tag{34}$$

where we will later replace $k_x := \Delta\beta_x = -\left(\beta_{\mathrm{x,in}} - \beta_{\mathrm{x,out}}\right)$ and $k_y := \Delta\beta_y = -\left(\beta_{y,\mathrm{in}} - \beta_{y,\mathrm{out}}\right)$. For the Fourier transforms of the perturbation and the shape functions we use the notations: $\hat{f}\left(k_x,k_y\right)$, $\hat{s}\left(k_x,k_y\right)$ respectively.

The convolution theorem for the definition of the two dimensional Fourier transform given in Eqn. (34) states that

$$\mathscr{F}\{f(x,y)s(x,y)\}\left(k_x,k_y\right) = \frac{1}{4\pi^2}\left(\hat{f}\left(k_x,k_y\right) * \hat{s}\left(k_x,k_y\right)\right). \tag{35}$$

The diffraction efficiency of a perturbation $f(x,y)$ with the shape $s(x,y)$ (Eqn. (33)) can now be written as

$$\frac{P_{\mathrm{out}}}{P_{\mathrm{in}}} = \hat{K}^2\left|\frac{1}{4\pi^2}\hat{f}\left(k_x,k_y\right) * \hat{s}\left(k_x,k_y\right)\right|^2. \tag{36}$$

The Fourier transform of a periodic perturbation function can be expressed as a sum of delta functions (sinusoids in real space), which are the identity of the convolution operation. Therefore, for periodic perturbations Eqn. (36) can be written in the following form

$$\frac{P_{\mathrm{out}}}{P_{\mathrm{in}}} = \hat{K}^2 p_m^2 a_m^2 A^2 {p_s}^2\left(\Delta\beta_x - \frac{2\pi}{\Lambda}, \Delta\beta_y\right), \tag{37}$$

where $A$ is the area, $a_m$ is the average height of the modulation, $p_m$ is the structure factor of the modulation and $p_s\left(\Delta\vec{\beta}\right) \equiv \hat{s}\left(\Delta\vec{\beta}\right)/A$ is the structure factor of the shape, which tends to $p_s\left(\Delta\beta_x - \frac{2\pi}{\Lambda} \to 0, \Delta\beta_y \to 0\right) \to 1$ when the diffraction condition is exactly met. $a_m = \frac{\int\int_A f(x,y)dxdy}{A}$ and $p_m = \frac{\int\int_A \sin\left(\vec{\beta}_g\cdot\vec{r}\right)f(x,y)dxdy}{\int\int_A f(x,y)dxdy}$ are defined for $f(x,y)$ in a similar fashion as $\Gamma_{\mathrm{tot}}$ and $\eta_{[\mathrm{A}]}$ for $\Gamma(x,y)$. Eqn. (37) can therefore be written in terms of $\Gamma_{\mathrm{tot}}$ and

$\eta_{[A]}$. The conversion is explained in Supplementary Section IV. In terms of mass distributions Eqn. (37) reads

$$\frac{P_{\text{out}}}{P_{\text{in}}} = 4|K|^2 n_c^2 \left(\frac{dn}{dc}\right)^2 \eta_{[A]}^2 \Gamma_{\text{tot}}^2 A^2 {p_s}^2 \left(\Delta\beta_x - \frac{2\pi}{\Lambda}, \Delta\beta_y\right). \tag{38}$$

Eqns. (37) and (38) are useful to estimate the sharpness of the resonance condition and enable to estimate the noise rejection capabilities of the diffraction grating. The sharpness of the resonance is fully determined by the structure factor of the shape.

While Eqn. (37) is convenient to evaluate, it might be beneficial for some readers to directly see an algebraic manipulation of Eqn. (36). We will do this in the following two subsections taking the example of a sinusoidal perturbation with two different shape functions. For the sinusoidal perturbation described in the next section Eqn. (37) reads ($p_m = 0.5$ and $a_m = \frac{t_m}{2}$)

$$\frac{P_{\text{out}}}{P_{\text{in}}} = \hat{K}^2 \frac{t_m^2}{16} A^2 {p_s}^2 \left(\Delta\beta_x - \frac{2\pi}{\Lambda}, \Delta\beta_y\right). \tag{39}$$

### 1. Example 1: Rectangular grating area with sinusoidal perturbation

Let us consider a sinusoidal grating with grating normal along the $x$ coordinate, grating period $\Lambda$, amplitude $\frac{t_m}{2}$ and offset $\frac{t_m}{2}$, restricted to a rectangular shape with length $L_x$ and $L_y$. The perturbation and shape functions are defined by

$$f(x,y) = \left(\frac{t_m}{2} + \frac{t_m}{2}\sin\left(\frac{2\pi}{\Lambda}x\right)\right) \tag{40}$$

and

$$s(x,y) = \text{rect}\left(\frac{1}{L_x}x\right)\text{rect}\left(\frac{1}{L_y}y\right), \tag{41}$$

where the rect function is defined as follows:

$$\text{rect}(x) = \begin{cases} 1 & |x| < \frac{1}{2} \\ \frac{1}{2} & |x| = \frac{1}{2} \\ 0 & \text{otherwise.} \end{cases} \tag{42}$$

Since $f(x,y)$ and $s(x,y)$ are both separable with respect to Cartesian coordinates, the diffracted power can be written as a product of two one-dimensional convolutions,

$$\frac{P_{\text{out}}}{P_{\text{in}}} = \hat{K}^2 \left|\frac{1}{4\pi^2}\left(\hat{f}_x(k_x) * \hat{s}_x(k_x)\right)\left(\hat{f}_y(k_y) * \hat{s}_y(k_y)\right)\right|^2. \tag{43}$$

With our definition of the Fourier transform, the transform pairs for constants, sinusoidal and rectangular functions read

$$1 \quad \circ\!\!-\!\!\bullet \quad 2\pi\delta(k_x) \tag{44}$$

$$\sin(ax) \quad \circ\!\!-\!\!\bullet \quad -i\pi\left(\delta(k_x - a) - \delta(k_x + a)\right) \tag{45}$$

$$\text{rect}(ax) \quad \circ\!\!-\!\!\bullet \quad \frac{1}{|a|}\text{sinc}\left(\frac{k_x}{2\pi a}\right), \tag{46}$$

where we used the definition of the normalized sinc function $\text{sinc}(\text{x}) = \frac{\sin(\pi\text{x})}{\pi\text{x}}$. Applying these relations, the Fourier transforms of the separated functions are

$$\hat{s}_x(\Delta\beta_x) = L_x\text{sinc}\left(\frac{L_x}{2\pi}\Delta\beta_x\right) \tag{47}$$

$$\hat{s}_y(\Delta\beta_y) = L_y\text{sinc}\left(\frac{L_y}{2\pi}\Delta\beta_y\right) \tag{48}$$

$$\hat{f}_x(\Delta\beta_x) = i\pi\frac{t_m}{2}\delta\left(\Delta\beta_x - \frac{2\pi}{\Lambda}\right) \tag{49}$$

$$\hat{f}_y(\Delta\beta_y) = 2\pi\delta(\Delta\beta_y). \tag{50}$$

Due to the shifting property of the convolution we can write

$$\begin{aligned} &\hat{s}_x\{\Delta\beta_x\} * \hat{f}_x\{\Delta\beta_x\} \\ &\quad = \text{sinc}\left(\frac{L_x}{2\pi}\Delta\beta_x\right) * i\pi\frac{t_m}{2}\delta\left(\Delta\beta_x - \frac{2\pi}{\Lambda}\right) \\ &\quad = i\pi\frac{t_m}{2}L_x\text{sinc}\left(\frac{L_x}{2\pi}\left(\Delta\beta_x - \frac{2\pi}{\Lambda}\right)\right). \end{aligned} \tag{51}$$

and

$$\begin{aligned} \hat{s}_y\{\Delta\beta_y\} * \hat{f}_y\{\Delta\beta_y\} &= L_y 2\pi\left(\text{sinc}\left(\frac{L_y}{2\pi}\Delta\beta_y\right) * \delta(\Delta\beta_y)\right) \\ &= 2\pi L_y\text{sinc}\left(\frac{L_y}{2\pi}\Delta\beta_y\right). \end{aligned} \tag{52}$$

Substituting this into Eqn. (43) results in the diffraction efficiency in the form of Eqn. (39) for a general detuning

$$\begin{aligned} \frac{P_{\text{out}}}{P_{\text{in}}} &= \hat{K}^2\frac{t_m^2}{16}A^2{p_s}^2\left(\Delta\beta_x - \frac{2\pi}{\Lambda}, \Delta\beta_y\right) \\ &= \frac{\hat{K}^2}{16}t_m^2 L_x^2 L_y^2 \\ &\quad \text{sinc}^2\left(\frac{L_x}{2\pi}\left(\Delta\beta_x - \frac{2\pi}{\Lambda}\right)\right)\text{sinc}^2\left(\frac{L_y}{2\pi}\Delta\beta_y\right). \end{aligned} \tag{53}$$

When $\Delta\beta_x \to \frac{2\pi}{\Lambda}$ and $\Delta\beta_y \to 0$ we have maximal coupling and Eqn. (53) simplifies to

$$\frac{P_{\text{out}}}{P_{\text{in}}} = \frac{\hat{K}^2}{16}t_m^2 L_x^2 L_y^2. \tag{54}$$

### 2. Example 2: Circular grating area with sinusoidal perturbation

Let us consider a sinusoidal grating with grating normal along the $x$ coordinate, grating period $\Lambda$, amplitude $\frac{t_m}{2}$ and offset $\frac{t_m}{2}$, restricted to a circular shape with diameter $D$,

$$f(x,y) = \left(\frac{t_m}{2} + \frac{t_m}{2}\sin\left(\frac{2\pi}{\Lambda}x\right)\right) \tag{55}$$

and

$$s(x,y) = \operatorname{circ}\left(\frac{2\sqrt{x^2+y^2}}{D}\right). \tag{56}$$

Here the circ function is defined as

$$\operatorname{circ}(r) = \begin{cases} 1 & r < \frac{1}{2} \\ \frac{1}{2} & r = \frac{1}{2} \\ 0 & \text{otherwise}, \end{cases} \tag{57}$$

with $r = \sqrt{x^2+y^2}$.

The Fourier transform of the perturbation is the same as in Supplementary Information Section II A 1

$$\hat{f}(\Delta\beta_x, \Delta\beta_y) = i\pi^2 t_m \delta\left(\Delta\beta_x - \frac{2\pi}{\Lambda}\right)\delta(\Delta\beta_y). \tag{58}$$

For $s(x,y)$ we perform a coordinate transformation into polar coordinates such that

$$s(r,\phi) = \operatorname{circ}\left(\frac{2r}{D}\right). \tag{59}$$

Due to the radial symmetry of the circ function we can apply the Fourier-Bessel transform

$$\hat{s}(k_r) := \mathscr{B}\{s(r,\phi)\}(k_r) = 2\pi\int_0^\infty \operatorname{circ}\left(\frac{2r}{D}\right) r J_0(rk_r)\,dr, \tag{60}$$

where $k_r = \sqrt{{k_x}^2+{k_y}^2}$. The Fourier Bessel Transform of the circular shape function with radius 1 reads [8]

$$\mathscr{B}\{\operatorname{circ}(r)\}(k_r) = 2\pi\int_0^1 \operatorname{circ}(r) r J_0(rk_r)\,dr = 2\pi\frac{J_1(k_r)}{k_r}. \tag{61}$$

By using the scaling property of the Fourier Bessel Transform $\mathscr{B}\{g(ar)\}(k_r) = \frac{1}{a^2}G\left(\frac{k_r}{a}\right)$, we obtain with $a = \frac{2}{D}$ the Fourier Bessel transform of the circular shape function with diameter $D$.

$$\hat{s}(\Delta\beta_r) = \frac{\pi D^2}{2}\frac{J_1\left(D\frac{\Delta\beta_r}{2}\right)}{\frac{D\Delta\beta_r}{2}} = \frac{\pi D^2}{4}2\frac{J_1\left(D\frac{\Delta\beta_r}{2}\right)}{\frac{D\Delta\beta_r}{2}}, \tag{62}$$

where $\Delta\beta_r = \sqrt{{\Delta\beta_x}^2+{\Delta\beta_y}^2}$. The reason for the factorisation of $\frac{1}{2}$ will become apparent later. Eqn. (62) can be transformed to Cartesian coordinates

$$\hat{s}(\Delta\beta_x, \Delta\beta_y) = \frac{\pi D^2}{4}2\frac{J_1\left(D\frac{\sqrt{\Delta\beta_x^2+\Delta\beta_y^2}}{2}\right)}{\frac{D\sqrt{\Delta\beta_x^2+\Delta\beta_y^2}}{2}}. \tag{63}$$

The convolution between the Fourier transform of the perturbation Eqn. (58) and the Fourier transform of the shape function Eqn. (63) can be determined with the shifting property of the convolution

$$\hat{s}(\Delta\beta_x, \Delta\beta_y) * \hat{f}(\Delta\beta_x, \Delta\beta_y) = i\pi^2 t_m \frac{\pi D^2}{4}2\frac{J_1\left(\frac{D}{2}\sqrt{\left(\Delta\beta_x - \frac{2\pi}{\Lambda}\right)^2+\Delta\beta_y^2}\right)}{\frac{D}{2}\sqrt{\left(\Delta\beta_x - \frac{2\pi}{\Lambda}\right)^2+\Delta\beta_y^2}}. \tag{64}$$

By inserting into Eqn. (36) we get the diffraction efficiency in the form of Eqn. (39)

$$\frac{P_{\text{out}}}{P_{\text{in}}} = \hat{K}^2\frac{t_m^2}{16}A^2{p_s}^2\left(\Delta\beta_x - \frac{2\pi}{\Lambda}, \Delta\beta_y\right) = \frac{\hat{K}^2}{16}t_m^2\left(\frac{\pi D^2}{4}\right)^2\left(2\frac{J_1\left(\frac{D}{2}\sqrt{\left(\Delta\beta_x - \frac{2\pi}{\Lambda}\right)^2+\Delta\beta_y^2}\right)}{\frac{D}{2}\sqrt{\left(\Delta\beta_x - \frac{2\pi}{\Lambda}\right)^2+\Delta\beta_y^2}}\right)^2. \tag{65}$$

When $\Delta\beta_x \to \frac{2\pi}{\Lambda}, \Delta\beta_y \to 0$, $2\frac{J_1\left(\frac{D}{2}\sqrt{\left(\Delta\beta_x - \frac{2\pi}{\Lambda}\right)^2+\Delta\beta_y^2}\right)}{\frac{D}{2}\sqrt{\left(\Delta\beta_x - \frac{2\pi}{\Lambda}\right)^2+\Delta\beta_y^2}} \to 1$ we have maximum coupling and Eqn. (39) reduces to

$$\frac{P_{\text{out}}}{P_{\text{in}}} = \frac{\hat{K}^2}{16}t_m^2\left(\frac{\pi D^2}{4}\right)^2. \tag{66}$$

## B. Random perturbation function - e.g. surface roughness

The diffraction efficiency for a random perturbation function is evaluated more conveniently using Eqn. (31), which can be written as

$$\frac{P_{\text{out}}}{P_{\text{in}}} = A\hat{K}^2\int_{-\infty}^{\infty}\int_{-\infty}^{\infty} g(u,v)\, e^{i\left(\vec{\beta}_{\text{in}}-\vec{\beta}_{\text{out}}\right)\cdot(u,v)}dudv \tag{67}$$

if the auto-correlation function

$$g(u = x-x', v = y-y') = \langle f(x,v)f(x',v')\rangle \tag{68}$$

decays rapidly within the area of interest $A$ (see Ref. [1]). Evaluating the scalar product in the exponent

and using the definitions $\Delta\beta_x = -(\beta_{\mathrm{x,in}} - \beta_{\mathrm{x,out}})$ and $\Delta\beta_y := -(\beta_{y,\mathrm{in}} - \beta_{y,\mathrm{out}})$ we obtain

$$\frac{P_{\mathrm{out}}}{P_{\mathrm{in}}} = A\hat{K}^2 \int_{-\infty}^{\infty}\int_{-\infty}^{\infty} g(u,v)\, e^{-i(\Delta\beta_x u + \Delta\beta_y v)} du dv. \tag{69}$$

Next, a transformation to polar coordinates is performed in real space

$$u = r\cos(\phi) \quad v = r\sin(\phi) \tag{70}$$

and frequency space

$$\Delta\beta_x = \frac{2\pi}{\Lambda}\cos(\vartheta) \quad \Delta\beta_y = \frac{2\pi}{\Lambda}\sin(\vartheta). \tag{71}$$

We assume that the wavevector difference $\Delta\vec{\beta}$ equals the grating vector $\vec{\beta}_g$ with modulus $\left|\Delta\vec{\beta}\right| = \left|\vec{\beta}_g\right| = 2\pi/\Lambda$ as this is the spatial frequency of interest

$$\frac{2\pi}{\Lambda} = \sqrt{\Delta\beta_x^2 + \Delta\beta_y^2} \quad \vartheta = \arctan\left(\frac{\Delta\beta_x}{\Delta\beta_y}\right). \tag{72}$$

The polar transformation of Eqn. (69) is

$$\frac{P_{\mathrm{out}}}{P_{\mathrm{in}}} = A\hat{K}^2 \int_0^{2\pi}\int_0^{\infty} g(r,\phi)\, e^{-ir\frac{2\pi}{\Lambda}(\cos(\vartheta)\cos(\phi)+\sin(\vartheta)\sin(\phi))} r dr d\phi. \tag{73}$$

Assuming a rotationally invariant autocorrelation function $g(u,v) = g_r\left(\sqrt{u^2+v^2}\right)$ we obtain the scattering efficiency

$$\frac{P_{\mathrm{out}}}{P_{\mathrm{in}}} = 2\pi A\hat{K}^2 \int_0^{\infty} g_r(r)\, J_0\left(\frac{2\pi}{\Lambda} r\right) r dr, \tag{74}$$

where $J_0$ is the zero'th order Bessel function. For an exponentially decaying autocorrelation function

$$g_r(r) = \sigma^2 e^{-(r/L_c)}, \tag{75}$$

the scattered power evaluates to

$$\frac{P_{\mathrm{out}}}{P_{\mathrm{in}}} = A\hat{K}^2 \frac{2\pi\sigma^2 L_c^2}{\left(1 + \left(\frac{2\pi}{\Lambda}\right)^2 L_c^2\right)^{3/2}}. \tag{76}$$

$\sigma$ is the root mean square of the surface's height fluctuations, and $L_c$ is their correlation length. Figure 5 illustrates surfaces with different $\sigma$ and $L_c$.

## III. NORMALIZATION OF BEAM ELECTRIC FIELDS FOR FREE SPACE AND GUIDED MODES (FOR USE IN EQN. (??))

In the following we describe the normalization of beam electric fields as needed to evaluate coupling constants in Eqn. (16). We use a distinct approaches for free space modes and for guided modes, respectively.

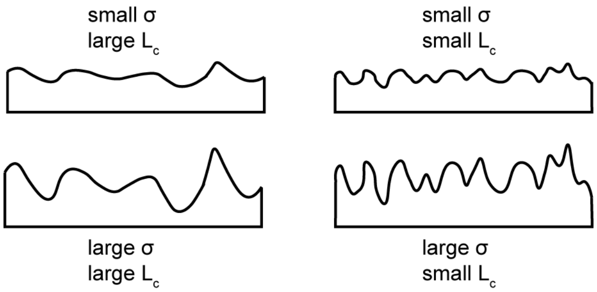


FIG. 5. Illustration of surfaces with different RMS roughness $\sigma$ and correlation lengths $L_c$

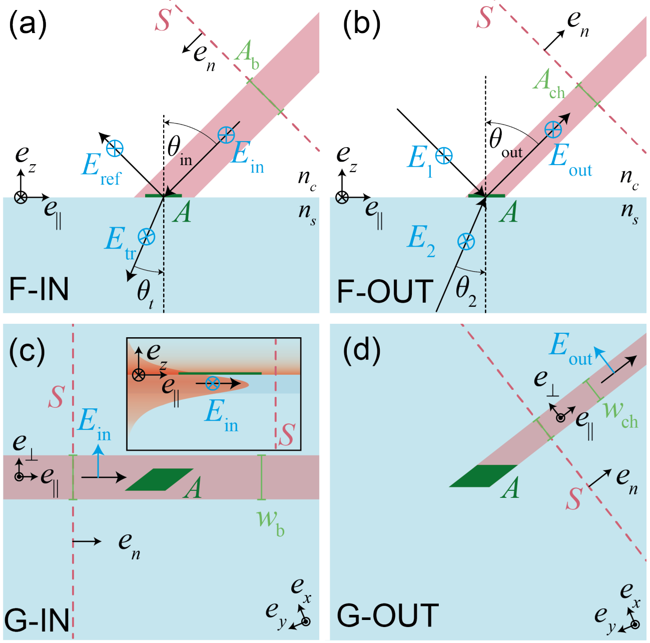


FIG. 6. Illustration of the geometry of incident and outgoing modes with TE polarization. (a) $\mathrm{F}_{c,\mathrm{in}}$ (b) $\mathrm{F}_{c,\mathrm{out}}$ (c) $\mathrm{G}_{\mathrm{in}}$ (d) $\mathrm{G}_{\mathrm{out}}$. The free space modes (a) and (b) consist of three beams: an incident, a reflected and a transmitted beam, or an outgoing and two incoming beams (with electric fields $E_1$ and $E_2$) respectively. The power flux in the far field is normalized to the power $P$. The field just above the interface is a superposition of the two beams propagating in the cover. Guided beams (c) and (d) are normalized following [1], which is extended to two dimensions by assuming a homogeneous intensity over the beam width. For the incident mode (c) the beam width is $w_b$. For the outgoing mode (d) the width is given by the orthogonal projection of the molecular grating onto the plane perpendicular to the propagation direction of the mode. We refer to it as characteristic grating width $w_{\mathrm{ch}}$. While in general the outgoing beam is non-uniform we show a set-up that yields a uniform outgoing beam. The direction of the grating normal is along the $x$-axis of the displayed coordinate system.

### A. Normalization of free spaces modes

For free space modes we distinguish between incident and outgoing modes. In both cases we compute the power flux through a plane $S$ (Figure 6a and b).

We evaluate Eqn. (25) assuming constant field strengths $\vec{E}_{\text{in/out}}$, $\vec{H}_{\text{in/out}}$ within the beam envelope such that

$$\begin{aligned} P &= \int\int_S \frac{1}{2}\vec{e}_n \cdot \left(\vec{E}_{\text{in/out}} \times \vec{H}^*_{\text{in/out}}\right) dS \\ &= \frac{1}{2} A_S \left(\vec{e}_n \cdot \left(\vec{E}_{\text{in/out},S} \times \vec{H}^*_{\text{in/out},S}\right)\right), \end{aligned} \tag{77}$$

where $A_S$ is the beam crosssection projected onto the plane $S$. $E_{\text{in/out},S}$ and $H_{\text{in/out},S}$ are the constant electric and magnetic field amplitudes of the incident/outgoing mode within the beam envelope evaluated on the plane $S$. This normalizes $E_{\text{in/out}}$ such that one can compute the normalized electric field on the surface.

With this normalization Table II is derived. We will show the normalization principle at the example of the TE polarized free space mode located on the cover side ($\text{F}_c$). The generalization to the $\text{F}_s$ case is straightforward. To derive the expressions for the TM polarization some adjustments are needed. These adjustments are indicated in the example for the TE case.

#### 1. Example normalization of $F_{\text{c,in}}$ for TE polarization

The beam $E_{\text{in}}$ carries power to the interface, while $E_{\text{ref}}$ and $E_{\text{tr}}$ carry power away (Figure 6a). Thus, the total incident power is described by $\text{E}_{\text{in},S}$. The beam envelope projected on $S$ has the area of the beam $A_b$. The normalized incident beam is not $\varphi$ dependent. Thus, Eqn. (77) can be written as

$$P = \frac{1}{2} A_{\text{b}} \frac{n_c}{Z_0} \left(\vec{e}_n \cdot \left(\vec{E}_{\text{in},S} \times \vec{e}_{\text{in}} \times \vec{E}^*_{\text{in},S}\right)\right). \tag{78}$$

$\vec{e}_{\text{n}} = (\sin(\theta_{\text{in}}), 0, -\cos(\theta_{\text{in}}))$ is the surface normal of the plane $S$ where the direction of $\vec{e}_n$ is chosen such that the Pointing flux is positive. $\vec{e}_{\text{in}} = (\sin(\theta_{\text{in}}), 0, -\cos(\theta_{\text{in}}))$ is the unit vector in propagation direction of the incident beam. The scalar and vector products can be evaluated and after solving for the field amplitude $E_{\text{in},S}$ we obtain

$$E_{\text{in},S} = \sqrt{\frac{2Z_0 P}{n_c A_{\text{b}}}}. \tag{79}$$

Obviously the normalization of the field strength in the incoming far-field is independent of the polarization. The field at the interface is equal to the vectorial sum of the incident and the reflected field. For TE modes all field vectors are collinear. Therefore, the tangential field of the normalized beam at the interface is

$$E_{\text{in,t}}(0) = \sqrt{\frac{2Z_0 P}{n_c A_{\text{b}}}} \left(1 + r^s_c\right). \tag{80}$$

For the TM mode the electric field vectors lie in the plane of incidence. Therefore, the electric field has both a tangential and a normal component. The fields of the incident and the reflected beam now have to be added as vectors, *i.e.* component-wise.

#### 2. Example normalization of $F_{\text{c,out}}$ for TE polarization

For an outgoing mode, the beam dimension is defined by the dimensions of the molecular grating (Figure 6b). Projected on the plane $S$ the beam has a crosssection $A_{\text{ch}} = A\cos(\theta_{\text{out}})$ (Figure 6b). Now the entire outgoing power is in the beam $E_{\text{out}}$. Evaluated on the plane $S$ Eqn. (77) yields

$$P = \frac{1}{2} A\cos(\theta_{\text{out}}) \frac{n_c}{Z_0} \left(\vec{e}_n \cdot \left(\vec{E}_{\text{out},S} \times \vec{e}_{\text{out}} \times \vec{E}^*_{\text{out},S}\right)\right). \tag{81}$$

$\vec{e}_{\text{n}} = (\sin(\theta_{\text{out}}), 0, \cos(\theta_{\text{in}}))$ is the surface normal of the plane $S$ where the direction of $\vec{e}_n$ is chosen such that the Pointing flux is positive. $\vec{e}_{\text{in}} = (\sin(\theta_{\text{out}}), 0, \cos(\theta_{\text{in}}))$ is the unit vector in propagation direction of the incident beam. The scalar and vector products can be evaluated and after solving for the field amplitude $E_{\text{out},S}$ we obtain

$$E_{\text{out},S} = \sqrt{\frac{2Z_0 P}{n_c A\cos(\theta_{\text{out}})}}. \tag{82}$$

Next, we use time reversal symmetry, which states that the field amplitudes do not change under time reversal. Therefore, $E_1$ and $E_2$ can be expressed with the Fresnel reflection and transmission coefficients of the interface

$$\begin{aligned} E_1 &= r^s_c(\theta_{\text{out}}) E_{\text{out}} \\ E_2 &= t^s_c(\theta_{\text{out}}) E_{\text{out}}. \end{aligned} \tag{83}$$

Eqns. (82) and (83) can be applied to the field amplitudes of the TM mode by replacing the Fresnel coefficients for TE with the ones for TM polarization. In the TE case, the field on the surface is equal to the sum of the outgoing and the field $E_1$ as all field vectors have the same orientation. Therefore, the normalized tangential field on the surface is

$$E_{\text{out,t}}(0) = \sqrt{\frac{2Z_0 P}{n_c A\cos(\theta_{\text{out}})}} \left(1 + r^s_c\right). \tag{84}$$

In the TM case, the tangential and normal components have to be considered separately as described at the end of Supplementary Information Section III A 1.

## B. Normalization of guided modes

The normalized field components on a waveguide surface for a guided mode in one dimension are given in Ref. [1]. We first state these equations in the notation used throughout this paper and then show how they can be generalized to two dimensions for an incident and outgoing mode.

### 1. TE Polarization

For TE polarization Ref. [1] states for the normalized electric field amplitude $A$,

$$A^2 = \frac{4\kappa^2\omega\mu_0 P_{1\mathrm{D}}}{(|\beta|\,(t_f + 1/\gamma + 1/\delta)\,(\kappa^2+\delta^2))}. \tag{85}$$

$t_f$ is the thickness of the waveguide,$\gamma, \delta, \kappa$ are the $z$-components of the wavevector in the three media (s,f,c) and are defined as: $\gamma = \frac{2\pi}{\lambda}\sqrt{N^2 - n_s^2}$, $\kappa = \frac{2\pi}{\lambda}\sqrt{n_f^2 - N^2}$, $\delta = \frac{2\pi}{\lambda}\sqrt{N^2 - n_c^2}$ [1]. Since the expression is for 1D problems $P_{1\mathrm{D}}$ is a power per length. By using the relations $\frac{\kappa^2}{\kappa^2+\delta^2} = \frac{n_f^2 - N^2}{n_f^2 - n_c^2}$, $t_{\mathrm{eff}} := (d + 1/\gamma + 1/\delta)$, $\frac{\omega\mu_0}{|\beta|} = \frac{Z_0}{N}$ and $\frac{\omega\varepsilon_0}{\beta} = \frac{1}{NZ_0}$ we arrive at the normalized tangential field component on the surface for 1D problems and TE polarization which reads

$$E_{\mathrm{t}}(0) = A = 2\sqrt{\frac{\left(n_f^2 - N^2\right) Z_0 P_{1\mathrm{D}}}{N\left(n_f^2 - n_c^2\right) t_{\mathrm{eff}}}}. \tag{86}$$

### 2. TM Polarization

For TM polarization Ref. [1] states for the normalized magnetic field amplitude $C$,

$$C^2 = \frac{4\omega\varepsilon_0 P_{1\mathrm{D}}}{|\beta|} n_f^2 n_c^4 \kappa^2 \left\{\left(n_c^4\kappa^2 + n_f^4\delta^2\right) t_{\mathrm{eff}}\right\}^{-1}. \tag{87}$$

mak with $t_{\mathrm{eff}} = t_f + \frac{n_s^2 n_f^2}{\gamma}\frac{\kappa^2+\gamma^2}{n_s^4\kappa^2 + n_f^4\gamma^2} + \frac{n_c^2 n_f^2}{\delta}\frac{\kappa^2+\delta^2}{n_c^4\kappa^2+n_f^4\delta^2}$. With some algebra it is possible to write $C$ in the notation of this paper ($C^2 = \frac{4}{NZ_0}\frac{n_c^2\left(n_f^2 - N^2\right)}{\left(n_f^2 - n_c^2\right)q_c}\frac{P}{t_{\mathrm{eff}}}$ with $q_c = \left(\frac{N}{n_f}\right)^2 + \left(\frac{N}{n_c}\right)^2 - 1$ (page 51 in [5])) and to compute the one dimensional tangential and normal field components according to $E_{\mathrm{t,1D}}(0) = \frac{i\delta}{n_c^2\omega\varepsilon_0}C$ and $E_{\mathrm{n,1D}}(0) = \frac{\beta}{n_c^2\omega\varepsilon_0}H_t(0) = \frac{\beta}{n_c^2\omega\varepsilon_0}C$ such that

$$E_{\mathrm{t}}(0) = i2\sqrt{\frac{\left(n_f^2 - N^2\right)}{N\left(n_f^2 - n_c^2\right)q_c}\frac{Z_0 P_{1\mathrm{D}}}{t_{\mathrm{eff}}}}\sqrt{\frac{N^2}{n_c^2} - 1} \tag{88}$$

and

$$E_{\mathrm{n}}(0) = 2\sqrt{\frac{\left(n_f^2 - N^2\right)}{N\left(n_f^2 - n_c^2\right)q_c}\frac{Z_0 P_{1\mathrm{D}}}{t_{\mathrm{eff}}}\frac{N}{n_c}}. \tag{89}$$

### 3. Normalization for incident guided modes

So far, we did not take into account the lateral extent of the beam, quoting the normalization of modes of infinite extent along $\vec{e}_\perp$. Since we assume rectangular beams with power uniformly distributed over its cross-section, the power unit length is simply given by $P_{1\mathrm{D}} = \frac{P}{w_b}$, which is to be substituted in the expressions (86), (89) and (88) for two-dimensional finite beams. (Figure 6c).

### 4. Normalization for outgoing guided modes

For the outgoing mode we choose the plane $S$ to be orthogonal to the propagation vector of the outgoing beam (Figure 6d). The beam has a width given by the orthogonal projection of the grating dimensions onto $S$, which we call the "characteristic grating width" $w_{\mathrm{ch}}$. In general, the outgoing beam has a nonuniform intensity distribution, even though there are set-ups that result in a uniform outgoing beam, such as the one shown in Figure 6d. Here we will approximate the beam as uniform. This implies a normalization given again by expressions (86), (89) and (88) with the substitution $P_{1\mathrm{D}} = \frac{P}{w_{\mathrm{ch}}}$.

## C. Azimuthal rotations of the plane of incidence and outgoing plane

So far we have not yet included rotations of the plane of incidence and outgoing plane around the $z$-axis. By definition the field for the TE polarization points in the positive $\vec{e}_\perp$ direction. Upon rotation, the tangential field component $E_{\mathrm{in,t}}(0)$ acquires an $x$- and a $y$-component in the coordinate system of the molecular grating. The components can be determined by the rotation matrix for positive rotations of the azimuth $\varphi$ around the $z$ axis

$$R = \begin{pmatrix} \cos(\varphi) & -\sin(\varphi) & 0 \\ \sin(\varphi) & \cos(\varphi) & 0 \\ 0 & 0 & 1. \end{pmatrix} \tag{90}$$

For our definition of the global coordinate system and an arbitrary $\varphi$ of the plane of incidence/outgoing plane (see Figure 3) the tangential components for the TE polarization read

$$\begin{aligned} E_x(0) &= -E_{\mathrm{t}}\sin(\varphi) \\ E_y(0) &= E_{\mathrm{t}}\cos(\varphi). \end{aligned} \tag{91}$$

This is valid for all incident and outgoing TE modes (F and G).

By definition, the tangential field of the TM modes points along $\vec{e}_{\parallel}$. Its direction (positive/negative) depends on whether the mode is incident or outgoing and whether it is located on the cover or substrate side (see Table II). Once the sign of $E_t$ is determined, the rotation around the $z$-axis results in

$$\begin{aligned} E_x(0) &= E_\mathrm{t}\cos(\varphi) \\ E_y(0) &= E_\mathrm{t}\sin(\varphi). \end{aligned} \tag{92}$$

## IV. CONVERSION OF MODULATED REFRACTIVE INDEX DIFFERENCE $\left(n_m^2 - n_c^2\right)$ TO COHERENT MASS DENSITY $\Gamma_\mathrm{coh}$

Coupled mode theory gives us an expression for the diffraction efficiency based on the refractive index of the perturbation $f(x,y)$. For diffractometric sensors, the property of interest is the coherent surface mass density $\Gamma_\mathrm{coh}$. We now show how to express the refractive index of a molecular grating in terms of the total mass of biomolecules. The height of the volume element that has an increased refractive index $n_m$ due to the presence of the biomolecule is described by the function $f(x,y)$. Therefore, the entire biomolecular mass on the pattern $m_\mathrm{tot} = \Gamma_\mathrm{tot}A$ is distributed in a volume $V = \iint\limits_A f(x,y)\,dxdy$, whereas $\Gamma_\mathrm{tot}$ is the total surface mass density and $A$ is the area of the pattern. Thus, the concentration of the biomolecules $c_P$ in the volume element can be expressed by

$$c_P = \frac{m_\mathrm{tot}}{V} = \frac{\Gamma_\mathrm{tot}A}{\int\int\limits_A f(x,y)\,dxdy}. \tag{93}$$

The connection between the refractive index of the volume element and the concentration of the biomolecules therein is [9]

$$\left(n_m^2 - n_c^2\right) = 2n_c\frac{dn}{dc}c_P. \tag{94}$$

By using Eqn. (93) and Eqn. (94) we obtain

$$\Gamma_\mathrm{tot} = \frac{\left(n_m^2 - n_c^2\right)}{2n_c\frac{dn}{dc}}\frac{\int\int\limits_A f(x,y)\,dxdy}{A}, \tag{95}$$

for the connection between total mass density and the perturbation function. From this and our assumption of a constant $n_m$ it follows that the perturbation function $f(x,y)$ and the mass density $\Gamma(x,y)$ are linked as

$$\Gamma(x,y) = \frac{\left(n_m^2 - n_c^2\right)}{2n_c\frac{dn}{dc}}f(x,y). \tag{96}$$

Finally, by using the definition of the analyte efficiency (Eqn. (4)), we can write the connection between the coherent surface mass density $\Gamma_\mathrm{coh}$ and the perturbation function $f(x,y)$ with constant refractive index $n_m$ as

$$\Gamma_\mathrm{coh} = \frac{\left(n_m^2 - n_c^2\right)}{2n_c\frac{dn}{dc}}\frac{\int\int\limits_A \sin\left(\vec{\beta}_g\cdot\vec{r}\right)f(x,y)\,dxdy}{A}. \tag{97}$$

## V. TM COUPLING COEFFICIENTS FOR THE THREE ARRANGEMENTS DESCRIBED IN TABLE

For completeness, we also computed the TM coupling coefficients (Table 3) for the three cases in Table . For the chosen observation direction, free space modes yield lower coupling coefficients for TM than for TE polarization. In the GG case, TM coupling is slightly larger for the chosen geometry. In conclusion, the difference is not large but as soon as free space modes are involved TE polarization should be favored, whereas for GG coupling one has to decide based on the angle $\varphi$, which polarization is to be favored.

## VI. QUANTIFICATION FORMULA FOR A NUMBER DENSITY OF PARTICLES WITH POLARIZABILITY $\alpha$

In some cases, for instance when the binding signal needs to be amplified by the binding of a nanoparticle, one might be interested in the number density of particles with radius $r_p$ made of a material with refractive index $n_p$ rather than the coherent mass density. By using the following definition for the polarizability: $\alpha = 4\pi r_p^3\frac{n_p^2-n_c^2}{n_p^2+2n_c^2}$ and the definition of the refractive index increment $\frac{dn}{dc} = \frac{3}{2}\frac{1}{\rho_p}n_c\frac{n_p^2-n_c^2}{n_p^2+2n_c^2}$ one can show that $\frac{dn}{dc} = \frac{\alpha n_c}{2\rho_p V_p}$, where $\rho_p$ is the density of the particle material and $V_p$ the particle volume. [10] We then can rewrite Eqn. (15) to directly compute the coherent particle number density $\sigma_\mathrm{p,coh}$ from the diffraction efficiency provided that the polarizability of the individual particles is known

$$\sigma_\mathrm{p,coh} = \frac{1}{|K|\,n_c^2\alpha A}\sqrt{\frac{P_\mathrm{out}}{P_\mathrm{in}}}. \tag{98}$$

Here we have used the relationship between the coherent number density of particles and the coherent mass density: $\Gamma_\mathrm{coh} = \sigma_\mathrm{p,coh}V_p\rho_p$.

| | | |
|---|---|---|
| $F_sF_s$ | $\left\lvert \frac{\pi}{\lambda n_s}\sqrt{\frac{1}{AA_b\cos(\theta_{\mathrm{out}})}}t_s^p\left(\theta_{\mathrm{in}}\right)t_s^p\left(\theta_{\mathrm{out}}\right)\left(\sqrt{1-\frac{n_s^2}{n_c^2}\sin^2\left(\theta_{\mathrm{in}}\right)}\sqrt{1-\frac{n_s^2}{n_c^2}\sin^2\left(\theta_{\mathrm{out}}\right)}+\frac{n_s^2}{n_c^2}\sin\left(\theta_{\mathrm{out}}\right)\sin\left(\theta_{\mathrm{in}}\right)\right)\right\rvert$ | 6.02e12 $\frac{1}{\mathrm{m}^3}$ |
| $GF_s$ | $\left\lvert \frac{\pi t_s^p(\theta_{\mathrm{out}})}{\lambda}\sqrt{\frac{\left(n_f^2-N^2\right)}{Nn_s\left(n_f^2-n_c^2\right)q_c}\frac{1}{t_{\mathrm{eff}}w_b}\frac{2}{A\cos(\theta_{\mathrm{out}})}}\left(i\sqrt{\frac{N^2}{n_c^2}-1}\sqrt{1-\frac{n_s^2}{n_c^2}\sin^2\left(\theta_{\mathrm{out}}\right)}+\frac{Nn_s}{n_c^2}\sin\left(\theta_{\mathrm{out}}\right)\right)\right\rvert$ | 3.58e14 $\frac{1}{\mathrm{m}^3}$ |
| GG | $\left\lvert \frac{2\pi}{\lambda}\frac{\left(n_f^2-N^2\right)}{N\left(n_f^2-n_c^2\right)q_c}\frac{1}{t_{\mathrm{eff}}\sqrt{w_b w_{\mathrm{ch}}}}\left(\left(\frac{N^2}{n_c^2}-1\right)\cos\left(2\varphi_{\mathrm{in}}\right)-\frac{N^2}{n_c^2}\right)\right\rvert$ | 1.78e16 $\frac{1}{\mathrm{m}^3}$ |

TABLE III. Coupling coefficient $|K|$ for coupling between two free space modes ($F_s/F_s$), a guided mode and a free space mode ($G/F_s$), and two guided modes (G/G) for TM polarized incident and outgoing beams. The following numerical values were substituted: $\lambda$: 635e-9 m, $n_s$: 1.521, $n_c$: 1.33, $n_f$: 2.117, $N$: 1.665, $A_b$: 7.9e-7 m$^2$ (circular beam of diameter 1e-3 m), $A$: 1.26e-7 m$^2$ (equivalent to a circular molecular grating of diameter 4e-4 m), $w_b$: 1e-3 m, $t_{\mathrm{eff}}$: 411e-9 m, $\theta_{\mathrm{in}}$: 70°, $|t_s^p(\theta_{\mathrm{in}})|$: 1.38, $\theta_{\mathrm{out}}$: 0°, $t_s^p(\theta_{\mathrm{out}})$: 1.07 (In the $GF_s$ case, this is the Fresnel coefficient of the three layer interface, but the numerical value is the same. (we used a thickness for the waveguide of $t_f$ = 145e-9 m), $\varphi_{\mathrm{in}}$ and $\varphi_{\mathrm{in}}$ are 0° for the first two cases where a free space mode is involved. In the GG case, we assume the grating to have the shape of a parallelogram with one of its sides being parallel to the propagation direction of the outgoing beam. This assures that the outgoing beam is uniform of width corresponding to the height of the parallelogram. We arbitrarily choose $\varphi_{\mathrm{in}} = 33.75°$, $\varphi_{\mathrm{out}} = -33.75°$. The characteristic width is simply the height of the parallelogram, which we took to be: $w_{\mathrm{ch}} = a\sin(2\varphi)$ =3.4e-4 m.

[1] D. Marcuse, *Theory of Dielectric Optical Waveguides.* Academic Press, 1974.

[2] For given $\vec{\beta}$, $k_z$ depends on the refractive medium. The relevant medium to consider is that from where an incident beam comes and into which an outgoing beam propagates, respectively.

[3] For the general case, where the coupling is not weak, as well as for details on the steps leading to Eqn. (23), we refer the reader to [1] Chapter 3.

[4] D. G. Hall, "I optical waveguide diffraction gratings: Coupling between guided modes," in *Progress in Optics* (E. Wolf, ed.), vol. 29, pp. 1–63, Elsevier, Jan. 1991.

[5] H. Kogelnik, "Theory of dielectric waveguides," in *Integrated Optics* (P. T. Tamir, ed.), Topics in Applied Physics, pp. 13–81, Springer Berlin Heidelberg, 1975.

[6] C. M. de Sterke and J. E. Sipe, "Ideal mode expansion for planar optical waveguides: application to the TM–TM coupling coefficient for grating structures," *J. Opt. Soc. Am. A, JOSAA*, vol. 7, pp. 636–645, Apr. 1990.

[7] Note that we normalize the total power $P$ of the beams (in units of [W]), in contrast to Ref. [1], where the beams were assumed to have infinite width in the $y$-direction, and normalization was to power per unit length in the direction transverse to the beam (with units $\left[\frac{\mathrm{W}}{\mathrm{m}}\right]$).

[8] J. W. Goodman, *Introduction to Fourier Optics.* Roberts and Company Publishers, 2005.

[9] C. Fattinger, "Focal molography: Coherent microscopic detection of biomolecular interaction," *Phys. Rev. X*, vol. 4, p. 031024, Aug. 2014.

[10] A. Frutiger, Y. Blickenstorfer, S. Bischof, C. Forró, M. Lauer, V. Gatterdam, C. Fattinger, and J. Vörös, "Principles for sensitive and robust biomolecular interaction analysis: The limits of detection and resolution of diffraction-limited focal molography," *Phys. Rev. Applied*, vol. 11, p. 014056, Jan. 2019.
